# Supplementary material for: Exploring the robust extrapolation of high-dimensional machine learning potentials
Source: arXiv:2112.10434 source file (2022-04-22)
Supplement: Supplementary file 1 [file dirac-rep.tex]

\usepackage{physics}
\usepackage{xparse}

% shortcuts for boldface and calligraphic

\newcommand{\mbf}[1]{\ensuremath{\mathbf{#1}}}

% a macro to typeset representations in bra-ket notation.
% can be used either with just ket \rep|A> or bra \rep<X|
% or together, \rep <X||A>
\NewDocumentCommand{\rep}{s d<| d|>}{%
% flips starring behavior relative to physics package 
\IfBooleanTF{#1}{
   \IfValueTF{#2}{
       \IfValueTF{#3}{\braket{#2}{#3}}{\bra{#2}}
       }{
       \IfValueTF{#3}{\ket{#3}}{}
       }
   }{
   \IfValueTF{#2}{
       \IfValueTF{#3}{\braket*{#2}{#3}}{\bra*{#2}}
       }{
       \IfValueTF{#3}{\ket*{#3}}{}
       }
   }
}

% for those who prefer the physics package \bra \ket notation
\NewDocumentCommand{\rbra}{sm}{\IfBooleanTF{#1}{\rep*<#2|}{\rep<#2|}}
\NewDocumentCommand{\rket}{sm}{\IfBooleanTF{#1}{\rep*|#2>}{\rep|#2>}}
\NewDocumentCommand{\rbraket}{smm}{\IfBooleanTF{#1}{\rep*<#2||#3>}{\rep<#2||#3>}}

% shortcut for CG "our way"

% macro to typeset a field. very flexible, should allow
% to describe non-symmetrized fields \field{\rho}
% fields that are symmetrized just once \field{\rho}x{\nu}
% equivariant fields \field[lambda mu]{\rho}x2
% and multi-scale LODE \field{\rho}x{\nu}[V]x{\nu'}
\NewDocumentCommand{\field}{o m e{_} e{^} o e{_} e{^}}{
% use overline if an otimes argument is specified, or if there is a double field entry
\IfValueTF{#5}{\overline{
  #2\IfValueT{#3}{_#3}\IfValueT{#4}{^{\otimes #4}} % first block
  \otimes 
  #5\IfValueT{#6}{_#6}\IfValueT{#7}{^{\otimes #7}} % second block
  \IfValueT{#1}{;#1}
}}{
  \IfValueTF{#4}{\overline{
     #2\IfValueT{#3}{_#3}\IfValueT{#4}{^{\otimes #4}}
     \IfValueT{#1}{;#1}
  }}
  {#2\IfValueT{#3}{_#3}}
}
}

% shortcuts for commonly-used fields
\NewDocumentCommand{\frho}{o e{_} e{^}}{
\field[#1]{\rho}_{#2}^{#3}
}

% shortcuts for commonly used feature indices

\newcommand{\e}{a}  % element index

% we use \bx for Cartesian basis, and \br to indicate atom positions

\newcommand{\bx}{\mbf{x}}

\NewDocumentCommand{\ex}{e_}{
\IfValueTF{#1}{\e_{#1}\bx_{#1}}{\e\bx}
}  % element index

% common indices for fully discretized density basis, and all sorts of combinations of subindices
\NewDocumentCommand{\lm}{e_}{
\IfValueTF{#1}{l_{#1}m_{#1}}{lm}
}
\NewDocumentCommand{\nlm}{e_}{
\IfValueTF{#1}{n_{#1}\lm_{#1}}{n\lm}
}
\NewDocumentCommand{\enlm}{e_}{
\IfValueTF{#1}{\e_{#1}\nlm_{#1}}{\e\nlm}
}
\NewDocumentCommand{\en}{e_}{
\IfValueTF{#1}{\e_{#1}n_{#1}}{\e n}
}
% coupled angular momentum basis
\NewDocumentCommand{\nlk}{e_}{
\IfValueTF{#1}{n_{#1}l_{#1}k_{#1}}{nlk}
}
\NewDocumentCommand{\enlk}{e_}{
\IfValueTF{#1}{\e_{#1}\nlk_{#1}}{\e\nlk}
}
\NewDocumentCommand{\enl}{e_}{
\IfValueTF{#1}{\en_{#1}l_#1}{\en l}
}
\NewDocumentCommand{\nl}{e_}{
\IfValueTF{#1}{n_{#1}l_#1}{n l}
}

% SOAP shortcuts - starred version removes ; separators
\NewDocumentCommand{\nnl}{s}{
\IfBooleanTF{#1}{n_1 n_2 l}{n_1; n_2; l}
}
\NewDocumentCommand{\ennl}{s}{
\IfBooleanTF{#1}{\en_1 \en_2 l}{\en_1; \en_2; l}
}

% greek indices for equivariants
\NewDocumentCommand{\gslm}{s}{
\IfBooleanTF{#1}{\sigma\lambda\mu}{\sigma;\lambda\mu}
}
