# Supplementary material for: Exploring the robust extrapolation of high-dimensional machine learning potentials
Source: arXiv:2112.10434 source file (2022-04-22)
Supplement: Supplementary file 2 [file defs.tex]

\input{dirac-rep}
\newcommand{\vv}[1]{\bm{#1}}
\newcommand{\strg}[1]{\mathrm{#1}}
\newcommand{\crl}[1]{\mathcal{#1}}

\newcommand{\density}[3]{ \braket*{#1}{#2}_{#3} }
\newcommand{\densitydag}[3]{  \braket*{#2}{#1}_{#3} }
\newcommand{\densitym}[4]{ \matrixel{#1}{#4}{#2}_{#3} }
\newcommand{\densitysqt}[3]{ \braket*{#1}{#2^{(2)}}_{#3} }
\newcommand{\densitysq}[3]{ \braket{#1}{#2^{(1)}}_{#3} }
\newcommand{\densitysqdag}[3]{  \braket{#2^{(1)}}{#1}_{#3} }
\newcommand{\densitycube}[3]{ \braket*{#1}{#2^{(2)}}_{#3} }

\newcommand{\smearing}[1]{g\left(#1\right)}
\newcommand{\gaus}[2]{\CN_{#2}\pqty\big{#1}}
\newcommand{\ddelta}[1]{\delta(#1)}

\newcommand{\xj}{\mathcal{X}_{j}}
\newcommand{\xk}{\mathcal{X}_{k}}
\newcommand{\bri}{\mathbf{r}_i}
\newcommand{\brj}{\mathbf{r}_j}
\newcommand{\brij}{\mathbf{r}_{ij}}

\newcommand{\bu}{\mathbf{u}}
\newcommand{\bk}{\mathbf{k}}
\newcommand{\bK}{\mathbf{K}}
\newcommand{\bt}{\mathbf{t}}
\newcommand{\by}{\mathbf{y}}
\newcommand{\bw}{\mathbf{w}}
\newcommand{\bz}{\mathbf{z}}
\newcommand{\That}{\hat{t}}
\newcommand{\Rhat}{\hat{R}}
\newcommand{\bPsi}{\mathbf{\Psi}}
\newcommand{\bPhi}{\mathbf{\Phi}}
\newcommand{\dint}{\textrm{d}}
\newcommand{\dbr}{\dint\br}
\newcommand{\dThat}{\dint\That}
\newcommand{\dRhat}{\dint\Rhat}
\newcommand{\drhat}{\dint\brhat}
\newcommand{\cald}{\mathcal{D}}
\newcommand{\calk}{\mathcal{K}}
\newcommand{\CB}{\mathcal{B}}
\newcommand{\CT}{\mathcal{T}}
\newcommand{\loss}{\ell}
\newcommand{\diag}{\ensuremath{\operatorname{diag}}}
\newcommand{\iket}[2]{\ket{#1}_{#2}}
\newcommand{\ibraket}[3]{\braket{#1}{#2}_{#3}}
\newcommand{\CN}{\mathcal{N}}
\newcommand{\sothree}{\ensuremath{\mathcal{SO}\left(3\right)}}
\newcommand{\othree}{\ensuremath{{\mathcal{O}\left(3\right)}}}
\newcommand{\behat}{\ensuremath{\hat{\mathbf{e}}}}
\newcommand{\angstrom}{\text{\AA}}

\newcommand{\D}[1]{\operatorname{d}{#1}} 
\newcommand{\gs}{\ensuremath{g_\text{s}}}
\newcommand{\gb}{\ensuremath{g_\text{b}}}
\newcommand{\nmax}{\ensuremath{n_\text{max}}}
\newcommand{\lmax}{\ensuremath{l_\text{max}}}

\newcommand{\DOS}{\mathrm{DOS}}
\newcommand{\LDOS}{\mathrm{LDOS}}
\newcommand{\LADOS}{\mathrm{LADOS}}
\newcommand{\Eband}{\epsilon_{\text{band}}}
\newcommand{\Efermi}{\epsilon_{F}}
